# Supplementary material for: EyeFormer: Predicting Personalized Scanpaths with Transformer-Guided Reinforcement Learning
Source: arXiv:2404.10163 source file (2024-04-21)
Supplement: Supplementary file 1 [file 10-Supp.tex]

\setlength{\tabcolsep}{2pt}
\def\w{0.1\linewidth}

 \centering
\begin{tabular}{c *9c}
\bf \begin{turn}{90} 
\bf \ \ \ \ \ \ \  \REVISION{Image}
\end{turn} & 
\includegraphics[height=\w, trim=10 10 10 10, clip]{source/figures/orig_images/eb06ec.jpg} &
\includegraphics[height=\w, trim=10 10 10 10, clip]{source/figures/orig_images/cd9e29.jpg} &
\includegraphics[height=\w, trim=16 20 16 10, clip]{source/figures/orig_images/46e638.jpg} &
\includegraphics[height=\w, trim=16 20 0 5, clip]{source/figures/orig_images/5db7bc.jpg} &
\includegraphics[height=\w, trim=10 10 10 5, clip]{source/figures/orig_images/9aabba.png} &
\includegraphics[height=\w, trim=10 10 10 0, clip]{source/figures/orig_images/e7a5c0.png} &
\includegraphics[height=\w, trim=16 20 16 15, clip]{source/figures/orig_images/b4a27a.png} &
\includegraphics[height=\w, trim=18 20 18 15, clip]{source/figures/orig_images/c6a6d9.png} 
\\
\bf \begin{turn}{90} 
\bf \ \ \ \ \ \ \ \ \  \REVISION{GT}
\end{turn} & 
\includegraphics[height=\w, trim=10 10 10 10, clip]{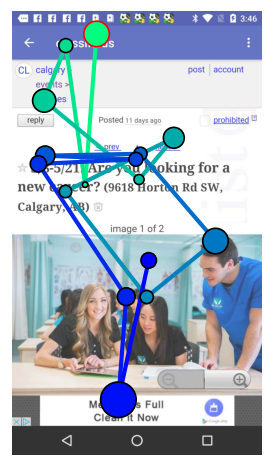} &
\includegraphics[height=\w, trim=10 10 10 10, clip]{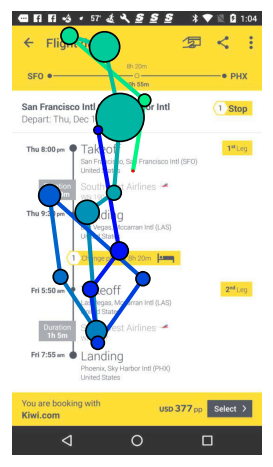} &
\includegraphics[height=\w, trim=16 20 16 10, clip]{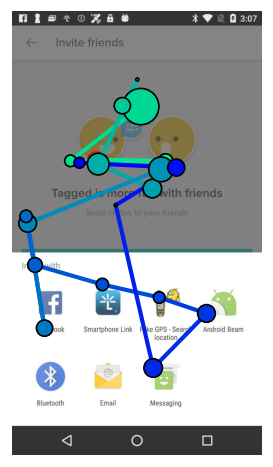} &
\includegraphics[height=\w, trim=16 20 0 5, clip]{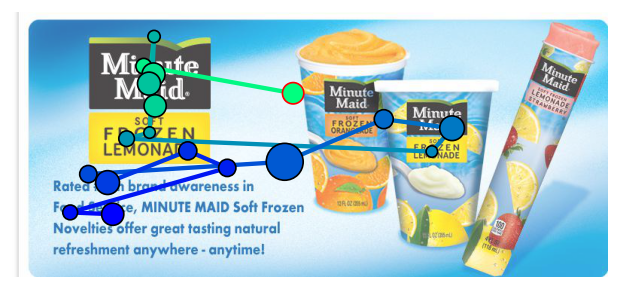} &
\includegraphics[height=\w, trim=10 10 10 5, clip]{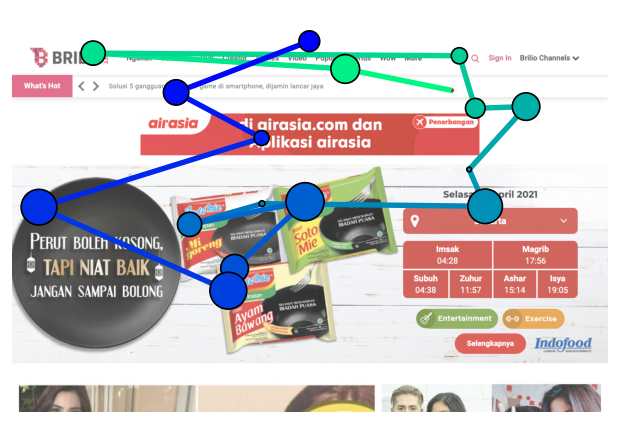} &
\includegraphics[height=\w, trim=10 10 10 0, clip]{source/figures/vertical_no_trans/e7a5c0_kh054_gt.png} &
\includegraphics[height=\w, trim=16 20 16 18, clip]{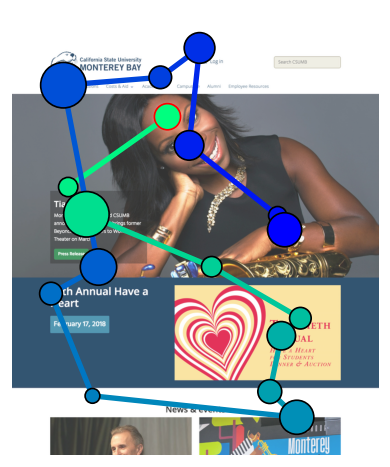} &
\includegraphics[height=\w, trim=18 20 18 18, clip]{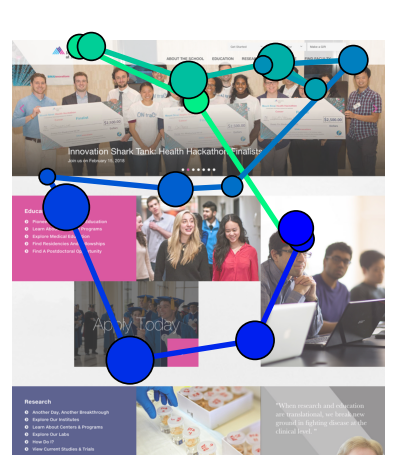} 
\\
\bf \begin{turn}{90} 
\bf \ \ \    \REVISION{\begin{tabular}{@{}c@{}}SaltiNet \\ on UEyes\end{tabular}} 
\end{turn} & 
\includegraphics[height=\w, trim=10 10 10 10, clip]{source/figures/comparison/351_test_scanpath_SaltiNet.png} &
\includegraphics[height=\w, trim=10 10 10 10, clip]{source/figures/comparison/375_test_scanpath_SaltiNet.png} &
\includegraphics[height=\w, trim=16 20 16 10, clip]{source/figures/comparison/2308_test_scanpath_SaltiNet.png} &
\includegraphics[height=\w, trim=16 20 0 5, clip]{source/figures/comparison/99142_test_scanpath_SaltiNet.png} &
\includegraphics[height=\w, trim=10 10 10 5, clip]{source/figures/comparison/brilio_test_scanpath_SaltiNet.png} &
\includegraphics[height=\w, trim=10 10 10 0, clip]
{source/figures/comparison/dayama13 (3)_test_scanpath_SaltiNet.png} &
\includegraphics[height=\w, trim=16 20 16 15, clip]{source/figures/comparison/ICWE_19_166_test_scanpath_SaltiNet.png} &
\includegraphics[height=\w, trim=18 20 18 15, clip]{source/figures/comparison/ICWE_19_392_test_scanpath_SaltiNet.png} 
\\
\bf \begin{turn}{90} 
\bf \  \REVISION{\begin{tabular}{@{}c@{}}DeepGaze III \\ Pretrained\end{tabular}}
\end{turn} & 
\includegraphics[height=\w, trim=10 10 10 10, clip]{source/figures/comparison/351_test_scanpath_DeepGazeIII.png} &
\includegraphics[height=\w, trim=10 10 10 10, clip]{source/figures/comparison/375_test_scanpath_DeepGazeIII.png} &
\includegraphics[height=\w, trim=16 20 16 10, clip]{source/figures/comparison/2308_test_scanpath_DeepGazeIII.png} &
\includegraphics[height=\w, trim=16 20 0 5, clip]{source/figures/comparison/99142_test_scanpath_DeepGazeIII.png} &
\includegraphics[height=\w, trim=10 10 10 5, clip]{source/figures/comparison/brilio_test_scanpath_DeepGazeIII.png} &
\includegraphics[height=\w, trim=10 10 10 0, clip]{source/figures/comparison/dayama13 (3)_test_scanpath_DeepGazeIII.png} &
\includegraphics[height=\w, trim=16 20 16 15, clip]{source/figures/comparison/ICWE_19_166_test_scanpath_DeepGazeIII.png} &
\includegraphics[height=\w, trim=18 20 18 15, clip]{source/figures/comparison/ICWE_19_392_test_scanpath_DeepGazeIII.png} 
\\

\bf \begin{turn}{90} 
\ \ \    \REVISION{\begin{tabular}{@{}c@{}}PathGAN \\ Pretrained\end{tabular}}
\end{turn} & 
\includegraphics[height=\w, trim=10 10 10 10, clip]{source/figures/comparison/351_ test_scanpath_PathGAN_Pretrained.png} &
\includegraphics[height=\w, trim=10 10 10 10, clip]{source/figures/comparison/375_ test_scanpath_PathGAN_Pretrained.png} &
\includegraphics[height=\w, trim=16 20 16 10, clip]{source/figures/comparison/2308_ test_scanpath_PathGAN_Pretrained.png} &
\includegraphics[height=\w, trim=16 20 0 5, clip]{source/figures/comparison/99142_ test_scanpath_PathGAN_Pretrained.png} &
\includegraphics[height=\w, trim=10 10 10 5, clip]{source/figures/comparison/brilio_ test_scanpath_PathGAN_Pretrained.png} &
\includegraphics[height=\w, trim=10 10 10 0, clip]{source/figures/comparison/dayama13 (3)_ test_scanpath_PathGAN_Pretrained.png} &
\includegraphics[height=\w, trim=16 20 16 15, clip]{source/figures/comparison/ICWE_19_166_ test_scanpath_PathGAN_Pretrained.png} &
\includegraphics[height=\w, trim=18 20 18 15, clip]{source/figures/comparison/ICWE_19_392_ test_scanpath_PathGAN_Pretrained.png}
\\
\bf \begin{turn}{90} 
\bf \ \ \ \  \REVISION{\begin{tabular}{@{}c@{}}PathGAN \\ on UEyes\end{tabular}}
\end{turn} & 
\includegraphics[height=\w, trim=10 10 10 10, clip]{source/figures/comparison/351_ test_scanpath_PathGAN_UEyes.png} &
\includegraphics[height=\w, trim=10 10 10 10, clip]{source/figures/comparison/375_ test_scanpath_PathGAN_UEyes.png} &
\includegraphics[height=\w, trim=16 20 16 10, clip]{source/figures/comparison/2308_ test_scanpath_PathGAN_UEyes.png} &
\includegraphics[height=\w, trim=16 20 0 5, clip]{source/figures/comparison/99142_ test_scanpath_PathGAN_UEyes.png} &
\includegraphics[height=\w, trim=10 10 10 5, clip]{source/figures/comparison/brilio_ test_scanpath_PathGAN_UEyes.png} &
\includegraphics[height=\w, trim=10 10 10 0, clip]{source/figures/comparison/dayama13 (3)_ test_scanpath_PathGAN_UEyes.png} &
\includegraphics[height=\w, trim=16 20 16 15, clip]{source/figures/comparison/ICWE_19_166_ test_scanpath_PathGAN_UEyes.png} &
\includegraphics[height=\w, trim=18 20 18 15, clip]{source/figures/comparison/ICWE_19_392_ test_scanpath_PathGAN_UEyes.png}
\\

\bf \begin{turn}{90} 
\bf \ \ \ \ \ \ \ \ \REVISION{\begin{tabular}{@{}c@{}}Ours\end{tabular}}
\end{turn} & 
\includegraphics[height=\w, trim=10 10 10 10, clip]{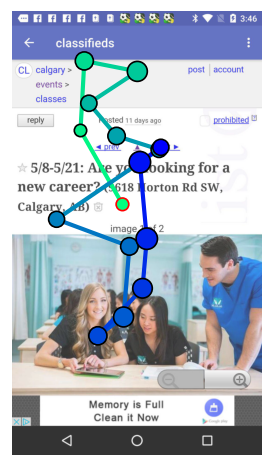} &
\includegraphics[height=\w, trim=10 10 10 10, clip]{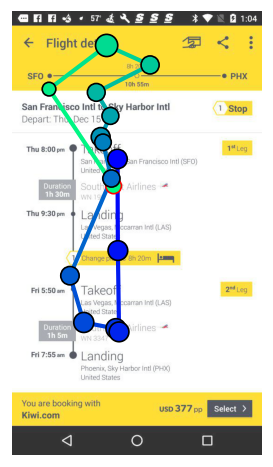} &
\includegraphics[height=\w, trim=16 20 16 10, clip]{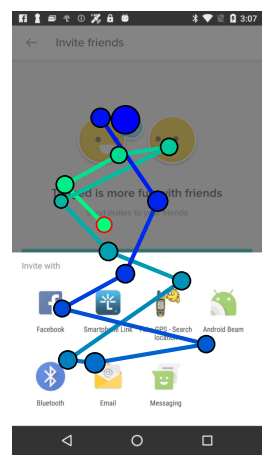} &
\includegraphics[height=\w, trim=16 20 0 5, clip]{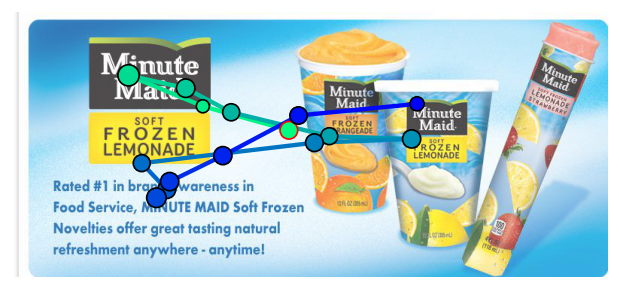} &
\includegraphics[height=\w, trim=10 10 10 5, clip]{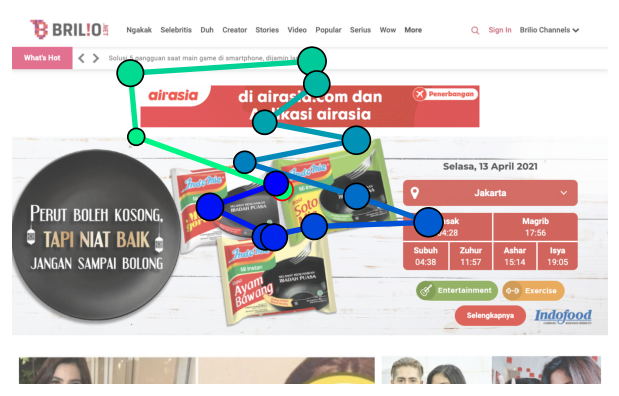} &
\includegraphics[height=\w, trim=10 10 10 0, clip]{source/figures/vertical_no_trans/e7a5c0_kh054_pred.png} &
\includegraphics[height=\w, trim=16 20 16 15, clip]{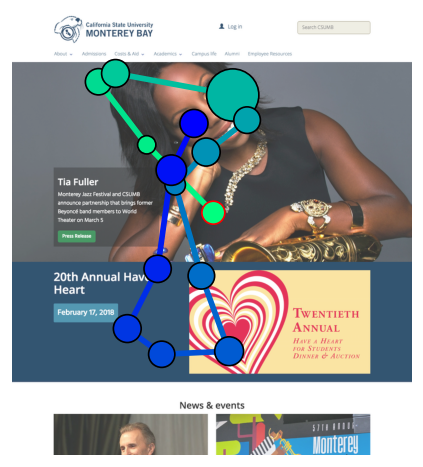} &
\includegraphics[height=\w, trim=18 20 18 15, clip]{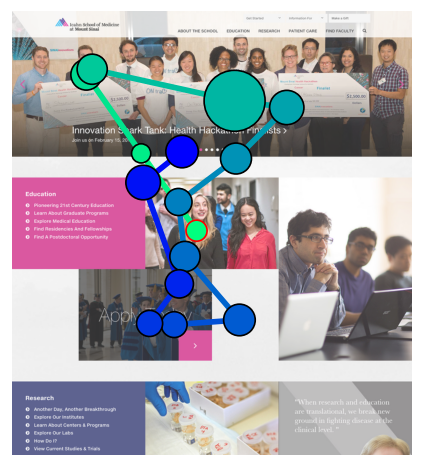} 
\\
\end{tabular}
\caption{
    Additional qualitative comparison. We compare and contrast different scanpath models. 
    Our model can predict more realistic scanpaths with more accurate fixation points than other models. 
}
\label{fig:scanpath_qualitative}
